# Supplementary material for: Overhead-Aware Distributed CSI Selection in the MIMO Interference Channel
Source: arXiv:1504.06794 source file (2015-07-06)
Supplement: Supplementary file 1 [file appendix.tex]

\appendices
\section{Proof of Proposition \ref{thm:grandCoal}}\label{proof:grandCoal}
